# Supplementary material for: Expert-Grounded Automatic Prompt Engineering for Extracting Lattice Constants of High-Entropy Alloys from Scientific Publications using Large Language Models
Source: arXiv:2512.22130 ancillary file (2025-12-05)
Supplement: Supplementary file 1 [file Supporting_Information.pdf]

**Supplementary Information for**  
**Expert-Grounded Automatic Prompt Engineering for Extracting**  
**Lattice Constants of High-Entropy Alloys from Scientific**  
**Publications using Large Language Models**

Shunshun Liu,<sup>1</sup> Talon R. Booth,<sup>1</sup> Yangfeng Ji,<sup>2</sup>  
Wesley Reinhart,<sup>3,4</sup> and Prasanna V. Balachandran<sup>1,\*</sup>

<sup>1</sup>*Department of Materials Science and Engineering,  
University of Virginia, Charlottesville, VA, USA*

<sup>2</sup>*Department of Computer Science, University of Virginia, Charlottesville, VA, USA*

<sup>3</sup>*Department of Materials Science and Engineering,  
Pennsylvania State University, State College, PA, USA*

<sup>4</sup>*Institute for Computational and Data Sciences,  
Pennsylvania State University, State College, PA, USA*

(Dated: November 20, 2025)

---

\* pvb5e@virginia.edu

## **S1. PROMPTS USED FOR CONSTRUCTING THE LLM APPLICATION SURVEY FIGURE**

The Figure S1 was created using data from the Ai2 Asta tool [1]. The following search terms were used:

- Find papers that use LLM in materials science
- Work harder
- Use the following categories: Knowledge Extraction & Curation, Property Prediction & Modeling, Materials & Molecular Design (Generative), Scientific Reasoning & Hypothesis Generation, Workflow Automation & Self-Driving Laboratories, Data Management & Knowledge Infrastructure, Education & Scientific Communication, can you count how many papers in each class?

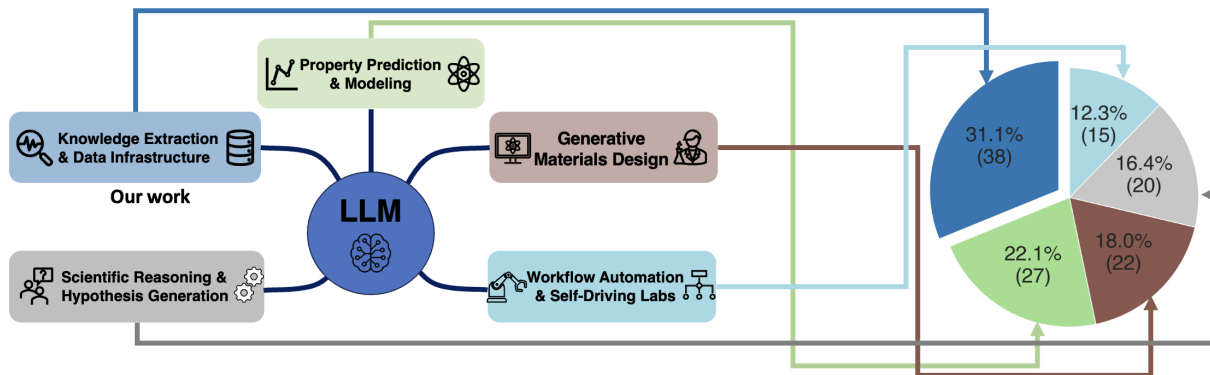

**Figure S1:** Applications of LLMs in materials science. Survey of 122 publications across five major application categories produced the following results. Knowledge Extraction and Data Infrastructure (31.1%) represents the most common use, involving automated knowledge and data extraction from scientific literature. Property Prediction and Modeling (22.1%) includes approaches for structure-property relationships. Generative Materials Design (18.0%) focuses on inverse design and computational generation of novel materials. Workflow Automation and Self-Driving Labs (16.4%) covers autonomous computational and experimental materials science. Scientific Reasoning and Hypothesis Generation (12.3%) addresses mechanistic understanding and identification of promising research directions. Source: Ai2-Asta [1].

## S2. PROMPTS USED IN THE PAPER FOR DATA EXTRACTION

```
1 Read the PDF file and extract required parameters.
2 You will ONLY report parameters of single phase high entropy alloy.
3 Lattice constant should be in the unit of angstrom, if lattice constant does not
  ↪ present, only report *None*.
4 The output MUST be in json format, follow the schema example:
5 {
6   "name": "Al0.25NbTiMoV"
7   "nominal_composition": "Al0.25Nb1.0Ti1.0Mo1.0V1.0",
8   "measured_composition": "Al5.4Ti22.0V22.1Nb25.5Mo25.0",
9   "lattice_constant": 3.206,
10  "phases": "BCC",
11  "alloy_condition": "As-cast",
12  "doi": "10.3390/e16020870"
13 }
```

---

**Figure S2:** Initial prompt for data extraction designed by the authors without any consultation with the LLM.

```

1 Read the PDF file and extract the following parameters for all high-entropy
  ↳ alloys discussed in the results section:
2
3 1. name (string, e.g., "AlCoCrFeNi")
4 2. nominal_composition (string, representing the stoichiometric ratio of each
  ↳ element, e.g., "Al1.0Co1.0Cr1.0Fe1.0Ni1.0". If an element's ratio is not
  ↳ explicitly stated, assume 1.0)
5 3. measured_composition (string, exactly as written in the paper)
6 4. lattice_constant (float, in angstroms, rounded to 3 decimal places)
7 5. phases (string, e.g., "BCC")
8 6. alloy_condition (string, e.g., "As-Cast")
9 7. doi (string)
10
11 Extract parameters primarily from the text. Use data from tables only if the text
  ↳ data is incomplete. Use figures as a last resort. If a parameter is truly
  ↳ missing from the PDF for a given alloy, explicitly report it as "Not found"
  ↳ rather than omitting it.
12
13 For each parameter, include a confidence score (0-100) indicating your certainty
  ↳ in the extracted information. Consider a score of 90 or above as high
  ↳ confidence.
14
15 The output should be a list of JSON objects, one for each alloy discussed in the
  ↳ paper, in the following format:
16
17 [
18   {
19     "name": "AlloyName",

```

```

20     "nominal_composition": "Element11.0Element21.0...",
21     "measured_composition": "Composition as written",
22     "lattice_constant": X.XXX,
23     "phases": "Phase1,Phase2,...",
24     "alloy_condition": "condition",
25     "doi": "DOI",
26     "confidence_scores": {
27         "name": XX,
28         "nominal_composition": XX,
29         "measured_composition": XX,
30         "lattice_constant": XX,
31         "phases": XX,
32         "alloy_condition": XX,
33         "doi": XX
34     }
35 },
36 ...
37 ]

```

39 Include an alloy in the output only if it is explicitly discussed in the results  
 ↳ section. Ensure that the output format and data closely match the provided  
 ↳ schema. If information for a specific parameter is not available, use "Not  
 ↳ found" and assign a low confidence score.

40

41 Example of correct output:

```

42 [
43     {
44         "name": "HfNbTaTiZr",
45         "nominal_composition": "Hf1.0Nb1.0Ta1.0Ti1.0Zr1.0",
46         "measured_composition": "Hf20.8Nb18.9Ta20.2Ti20.2Zr19.9",

```

```

47     "lattice_constant": 3.414,
48     "phases": "BCC",
49     "alloy_condition": "As-Cast",
50     "doi": "10.1016/j.jallcom.2014.11.064",
51     "confidence_scores": {
52         "name": 100,
53         "nominal_composition": 90,
54         "measured_composition": 95,
55         "lattice_constant": 100,
56         "phases": 100,
57         "alloy_condition": 95,
58         "doi": 100
59     }
60 }
61 ]
62
63 Example of output with missing data:
64 [
65     {
66         "name": "AlCoCrFeNi",
67         "nominal_composition": "Al1.0Co1.0Cr1.0Fe1.0Ni1.0",
68         "measured_composition": "Not found",
69         "lattice_constant": 3.567,
70         "phases": "FCC",
71         "alloy_condition": "Not found",
72         "doi": "10.1016/j.example.2023.01.001",
73         "confidence_scores": {
74             "name": 100,
75             "nominal_composition": 90,
76             "measured_composition": 0,

```

```
77         "lattice_constant": 95,  
78         "phases": 100,  
79         "alloy_condition": 0,  
80         "doi": 100  
81     }  
82 }  
83 ]
```

---

**Figure S3:** Optimized prompt from the TEXTGRAD output.

### S3. TEXT LOSS RETURNED FOR INDIVIDUAL PAPERS

```
1 Based on the evaluation criteria, here is my assessment of the output:
2 1. Does the output match the format provided in the question?
3 Yes, the output is a list of JSON objects matching the specified format.
4 2. Are the extracted materials high-entropy alloys?
5 No, these are not high-entropy alloys. They are ferritic alloys with G-phase
  ↪ precipitates.
6 3. Are the alloy compositions in the output correct and reflect the material?
7 Yes, the nominal compositions match those given in Table 1 of the paper.
8 4. Are the lattice constants in the output formatted in angstrom?
9 Yes, the lattice constants are given in angstroms (11.22 Å).
10 5. Are the lattice constants in the output truly the lattice constant of the
  ↪ material not others?
11 Yes, 11.22 Å matches the lattice parameter given for the Ni16Ti6Si7-G phase in
  ↪ Table 2.
12 6. Are the phase information in the output correct and reflect the material?
13 Yes, the phases listed (BCC, G-phase, L21) match those discussed in the paper.
14 7. Are the alloy conditions in the output correct and reflect the material?
15 Yes, the conditions listed (As-Cast, Solution-Treated, Cold-Rolled) are mentioned
  ↪ in the paper.
16 8. Is the DOI in the output matches with the original paper?
17 Yes, the DOI matches the one given at the top of the paper.
18 9. Is there any HEA high-entropy alloys missed in the provided output?
19 No, there are no high-entropy alloys discussed in this paper, so none are missed.
```

---

**Figure S4:** Text loss returned for Yang et al. [2] using the EvaluatePdfOutputLoss function.

```

1         I will evaluate the output according to the provided criteria:
2         1. Does the output match the format provided in the question?
3             Yes
4         2. Are the extracted materials high-entropy alloys?
5             No, the extracted alloy is described as a medium entropy alloy (MEA).
6         3. Are the alloy compositions in the output correct and reflect the material?
7             Yes
8         4. Are the lattice constants in the output formatted in angstrom?
9             Yes
10        5. Are the lattice constants in the output truly the lattice constant of the
        ↪ material not others?
11        No, the reported 10.9 Å is the lattice parameter of the Cr23C6 carbide, not the
        ↪ MEA matrix.
12        6. Are the phase information in the output correct and reflect the material?
13            Yes
14        7. Are the alloy conditions in the output correct and reflect the material?
15            Yes
16        8. Is the DOI in the output matches with the original paper?
17            Yes
18        9. Is there any HEA high-entropy alloys missed in the provided output?
19        No, the paper focuses on a medium entropy alloy, not a high entropy alloy.

```

---

**Figure S5:** Text loss returned for Pan et al. [3] using the EvaluatePdfOutputLoss function.

1 I will evaluate the output according to the provided criteria:

2 1. Does the output match the format provided in the question?

3 Yes, the output matches the JSON format specified in the question.

4 2. Are the extracted materials high-entropy alloys?

5 Yes, all extracted materials are high-entropy alloys from the FeCoCrAlNiTi<sub>x</sub>

↪ system.

6 3. Are the alloy compositions in the output correct and reflect the material?

7 Yes, the nominal and measured compositions appear to correctly reflect the

↪ materials described in the paper.

8 4. Are the lattice constants in the output formatted in angstrom?

9 The lattice constant is only provided for FeCoCrAlNiTi<sub>0.5</sub> and is in angstroms.

↪ For the others it's listed as "Not found".

10 5. Are the lattice constants in the output truly the lattice constant of the

↪ material not others?

11 The one lattice constant provided (11.303 Å for FeCoCrAlNiTi<sub>0.5</sub>) appears to be

↪ for the Ti<sub>2</sub>Ni phase rather than the overall alloy lattice constant.

12 6. Are the phase information in the output correct and reflect the material?

13 Yes, the phase information appears to be correct based on the description in the

↪ paper.

14 7. Are the alloy conditions in the output correct and reflect the material?

15 Yes, "As-Cast" is correct for these laser surface alloyed coatings.

16 8. Is the DOI in the output matches with the original paper?

17 Yes, the DOI matches the one given in the paper.

18 9. Is there any HEA high-entropy alloys missed in the provided output?

19 No, all FeCoCrAlNiTi<sub>x</sub> alloys discussed in the results section appear to be

↪ included.

---

**Figure S6:** Text loss returned for Wu et al. [4] using the EvaluatePdfOutputLoss function.



```
1           Here is my evaluation of the output:
2           1. Does the output match the format provided in the question? Yes
3           2. Are the extracted materials high-entropy alloys? No, this is described as a
           ↪ medium-entropy alloy.
4           3. Are the alloy compositions in the output correct and reflect the material?
           ↪ Yes, the nominal composition matches what is stated in the paper.
5           4. Are the lattice constants in the output formatted in angstrom? Yes
6           5. Are the lattice constants in the output truly the lattice constant of the
           ↪ material not others? No, the value given (0.255) appears to be the Burgers
           ↪ vector magnitude, not the lattice constant.
7           6. Are the phase information in the output correct and reflect the material? Yes,
           ↪ the phases listed match those described in the paper.
8           7. Are the alloy conditions in the output correct and reflect the material? Yes,
           ↪ the annealed condition is mentioned in the paper.
9           8. Is the DOI in the output matches with the original paper? Yes
10          9. Is there any HEA high-entropy alloys missed in the provided output? No, the
           ↪ paper focuses on this single medium-entropy alloy.
```

---

**Figure S7:** Text loss returned for Moon et al. [5] using the EvaluatePdfOutputLoss function.

```

1         I'll evaluate the output according to the provided criteria:
2         1. Does the output match the format provided in the question?
3         Yes, the output is a list of JSON objects with the specified fields.
4         2. Are the extracted materials high-entropy alloys?
5         Yes, both NiCuPdTiZrHf and NiCuTiZrHf are high-entropy alloys.
6         3. Are the alloy compositions in the output correct and reflect the material?
7         Yes, the nominal compositions match the information given in the paper.
8         4. Are the lattice constants in the output formatted in angstrom?
9         Yes, the lattice constant for NiCuPdTiZrHf is given in angstroms (0.319 Å).
10        5. Are the lattice constants in the output truly the lattice constant of the
        ↪ material not others?
11        Yes, the 0.319 Å value matches the B2 lattice constant reported in the paper for
        ↪ NiCuPdTiZrHf.
12        6. Are the phase information in the output correct and reflect the material?
13        Yes, the phases listed (B2, B19') match those discussed in the paper for these
        ↪ alloys.
14        7. Are the alloy conditions in the output correct and reflect the material?
15        Yes, the as-cast and homogenized conditions are correctly noted.
16        8. Is the DOI in the output matches with the original paper?
17        Yes, the DOI matches the one given in the paper.
18        9. Is there any HEA high-entropy alloys missed in the provided output?
19        No, the output covers the two main HEAs discussed in detail in the results
        ↪ section.

```

---

**Figure S8:** Text loss returned for Piorunek et al. [6] using the EvaluatePdfOutputLoss function.

1 I will evaluate the output according to the provided criteria:

2 1. Does the output match the format provided in the question?

3 Yes, the output matches the requested JSON format.

4 2. Are the extracted materials high-entropy alloys?

5 No, these are not high-entropy alloys. They are Mg-based alloys with Gd, Y, and  
 ↪ Zr additions.

6 3. Are the alloy compositions in the output correct and reflect the material?

7 Yes, the measured compositions match the data provided in Table 1 of the paper.

8 4. Are the lattice constants in the output formatted in angstrom?

9 Yes, the lattice constants are given in angstroms (e.g. 0.323 Å).

10 5. Are the lattice constants in the output truly the lattice constant of the  
 ↪ material not others?

11 Yes, the lattice constants match the 'a' parameter values given in Table 3 of the  
 ↪ paper.

12 6. Are the phase information in the output correct and reflect the material?

13 Yes, the phase information matches what is described in the paper for each  
 ↪ composition.

14 7. Are the alloy conditions in the output correct and reflect the material?

15 Yes, the alloy condition "As-deposited LDED" correctly reflects the laser  
 ↪ directed energy deposition process used.

16 8. Is the DOI in the output matches with the original paper?

17 Yes, the DOI matches the one given in the paper.

18 9. Is there any HEA high-entropy alloys missed in the provided output?

19 No, there are no high-entropy alloys in this paper, so none are missed.

---

**Figure S9:** Text loss returned for Jiang et al. [7] using the EvaluatePdfOutputLoss function.

```

1 I'll evaluate the output for each extracted material according to the provided
  ↳ criteria:
2     1. Does the output match the format provided in the question?
3     Yes. The output is a list of JSON objects with the required fields.
4     2. Are the extracted materials high-entropy alloys?
5     Yes. All extracted alloys are high-entropy alloys from the CoFeNiMnTixAl1-x
  ↳ system.
6     3. Are the alloy compositions in the output correct and reflect the material?
7     Yes. The compositions match those given in the paper for each alloy.
8     4. Are the lattice constants value in the output formatted in angstrom?
9     Yes. The lattice constants are given in angstroms.
10    5. Are the lattice constants in the output truly the lattice constant of the
  ↳ material not others?
11    Yes. The lattice constants match those reported in the paper for the BCC phase.
12    6. Are the phase information in the output correct and reflect the material?
13    Yes. The phase information matches what is reported in the paper for each
  ↳ composition.
14    7. Are the alloy conditions in the output correct and reflect the material?
15    Yes. The alloys are reported as "As-Cast" which matches the paper.
16    8. Is the DOI in the output matches with the original paper?
17    Yes. The DOI matches the one given in the paper.
18    9. Is there any HEA high-entropy alloys missed in the provided output?
19    Yes. The output is missing some of the intermediate compositions discussed in the
  ↳ paper, such as Ti0.1Al0.9, Ti0.3Al0.7, and Ti0.8Al0.2.

```

---

**Figure S10:** Text loss returned for Cui et al. [8] using the EvaluatePdfOutputLoss function.

#### **S4. PROMPT TRANSFERABILITY**

**TABLE S1:** Comparison of entity-level extraction performance across Claude 4.5 Sonnet, Gemini 2.5 Flash, and GPT-5 LLM models using the *initial prompt* with different thinking or reasoning configurations. Claude 4.5 Sonnet was tested with and without extended reasoning. When the extended reasoning capability was enabled, the thinking budget was set at 1024 tokens. Extended reasoning is disabled by default for Claude 4.5 Sonnet. Gemini 2.5 Flash was evaluated with and without dynamic reasoning (dynamic reasoning is the default configuration). GPT-5 was tested with minimal and medium reasoning budgets (medium reasoning is the default configuration). All models were evaluated using their default temperature settings.

(a) Claude 4.5 Sonnet variants

| Named Entity               | Claude 4.5 (extended reasoning) |        |          | Claude 4.5 (no reasoning) |        |          |
|----------------------------|---------------------------------|--------|----------|---------------------------|--------|----------|
|                            | Precision                       | Recall | F1 Score | Precision                 | Recall | F1 Score |
| Nominal composition        | 0.909                           | 1.000  | 0.952    | 0.667                     | 1.000  | 0.800    |
| Lattice constant           | 1.000                           | 1.000  | 1.000    | 0.733                     | 1.000  | 0.846    |
| Phase                      | 1.000                           | 1.000  | 1.000    | 0.733                     | 1.000  | 0.846    |
| Alloy processing condition | 1.000                           | 1.000  | 1.000    | 0.733                     | 1.000  | 0.846    |

(b) Gemini 2.5 Flash variants

| Named Entity               | Gemini 2.5 Flash (dynamic reasoning) |        |          | Gemini 2.5 Flash (no reasoning) |        |          |
|----------------------------|--------------------------------------|--------|----------|---------------------------------|--------|----------|
|                            | Precision                            | Recall | F1 Score | Precision                       | Recall | F1 Score |
| Nominal composition        | 1.000                                | 0.818  | 0.900    | 0.654                           | 0.773  | 0.708    |
| Lattice constant           | 1.000                                | 0.818  | 0.900    | 0.654                           | 0.773  | 0.708    |
| Phase                      | 1.000                                | 0.818  | 0.900    | 0.654                           | 0.773  | 0.708    |
| Alloy processing condition | 1.000                                | 0.818  | 0.900    | 0.654                           | 0.773  | 0.708    |

(c) GPT-5 variants

| Named Entity               | GPT-5 (medium reasoning) |        |          | GPT-5 (minimal reasoning) |        |          |
|----------------------------|--------------------------|--------|----------|---------------------------|--------|----------|
|                            | Precision                | Recall | F1 Score | Precision                 | Recall | F1 Score |
| Nominal composition        | 1.000                    | 0.864  | 0.927    | 0.850                     | 0.895  | 0.872    |
| Lattice constant           | 1.000                    | 0.864  | 0.927    | 1.000                     | 0.909  | 0.952    |
| Phase                      | 1.000                    | 0.864  | 0.927    | 1.000                     | 0.909  | 0.952    |
| Alloy processing condition | 1.000                    | 0.864  | 0.927    | 1.000                     | 0.909  | 0.952    |

**TABLE S2:** Comparison of data extraction performance across Claude 4.5 Sonnet, Gemini 2.5 Flash, and GPT-5 models using the *optimized prompt*. Precision and recall metrics were calculated with the same procedure as defined in Table 3. The best precision, recall, and F1 score is highlighted in bold font. The default configuration was used for all three LLM models: no reasoning for Claude 4.5 Sonnet, dynamic reasoning for Gemini 2.5 Flash and medium reasoning for GPT-5. The table also includes the cost (in USD) for processing the 46-publication set with each LLM, along with the cost-effectiveness ratio (average F1 score per dollar). Higher ratios indicate better extraction performance per unit cost.

**(a)** Claude 4.5 Sonnet no reasoning vs. Gemini 2.5 Flash dynamic reasoning vs. GPT-5 medium reasoning

| Named Entity             | Claude 4.5 (no reasoning) |              |              | Gemini 2.5 Flash (dynamic reasoning) |        |          | GPT-5 (medium reasoning) |        |          |
|--------------------------|---------------------------|--------------|--------------|--------------------------------------|--------|----------|--------------------------|--------|----------|
|                          | Precision                 | Recall       | F1 Score     | Precision                            | Recall | F1 Score | Precision                | Recall | F1 Score |
| As-cast single-phase BCC | <b>1.000</b>              | <b>0.977</b> | <b>0.988</b> | 0.951                                | 0.886  | 0.917    | 0.929                    | 0.886  | 0.907    |
| Nominal composition      | <b>0.977</b>              | <b>0.955</b> | <b>0.966</b> | 0.951                                | 0.886  | 0.917    | 0.905                    | 0.864  | 0.884    |
| Lattice constant         | <b>0.953</b>              | <b>0.932</b> | <b>0.942</b> | 0.951                                | 0.886  | 0.917    | 0.929                    | 0.886  | 0.907    |
| Approx. total cost (USD) |                           | 4.63         |              |                                      |        | 0.72     |                          | 2.62   |          |
| Average F1 Score / USD   |                           | 0.208        |              |                                      |        | 1.274    |                          | 0.343  |          |

**(b)** Claude 4.5 no reasoning vs. reasoning

| Named Entity             | Claude 4.5 (no reasoning) |              |              | Claude 4.5 (reasoning) |        |          |
|--------------------------|---------------------------|--------------|--------------|------------------------|--------|----------|
|                          | Precision                 | Recall       | F1 Score     | Precision              | Recall | F1 Score |
| As-cast single-phase BCC | <b>1.000</b>              | <b>0.977</b> | <b>0.988</b> | 0.955                  | 0.955  | 0.955    |
| Nominal composition      | <b>0.977</b>              | <b>0.955</b> | <b>0.966</b> | 0.955                  | 0.955  | 0.955    |
| Lattice constant         | <b>0.953</b>              | <b>0.932</b> | <b>0.942</b> | 0.932                  | 0.932  | 0.932    |
| Approx. total cost (USD) |                           | 4.63         |              |                        | 4.78   |          |
| Average F1 Score / USD   |                           | 0.208        |              |                        | 0.204  |          |

## S5. EXTENDED REASONING USING GEMINI 2.5 FLASH MODEL

```
1  **Initial Data Extraction and Analysis**
2  Alright, let's get down to business. My task is to meticulously extract specific
   ↪ information about high-entropy alloys (HEAs) from this document. I need to
   ↪ focus on the "Results and discussion" section, identifying each HEA and
   ↪ pulling out its name, nominal composition, measured composition, lattice
   ↪ constant, phases present, alloy condition, and the paper's DOI. I'll need to
   ↪ assign confidence scores to each piece of data, and if something's missing,
   ↪ I'll flag it as "Not found."
3  I'll start by systematically scanning the text. First, I'll hunt for HEA names.
   ↪ Then, for each HEA, I'll dig for the required parameters. The name is usually
   ↪ right there in the text. Nominal composition will be assumed equiatomic
   ↪ unless specified otherwise. Measured composition will be "Not found" unless
   ↪ precise percentages or ratios are given. Lattice constants will require
   ↪ finding Å values, ideally linked to diffraction data. Phases will be
   ↪ identified as "bcc," "fcc," etc. The alloy condition will be determined by
   ↪ looking for terms like "as-cast" or "annealed." Finally, the DOI is
   ↪ straightforward; it's the paper's unique identifier.
4  **Deep Dive into the Text**
5  Let's begin the search. I spot "TiVNbTa" and "TiVNbMoTa" right away in the first
   ↪ page's heading. That's a good start. I also see mentions of "bcc lattice"
   ↪ which tells me the phase of these alloys. Then, I found MoNbTaW and
   ↪ NiCoFeCrMn. "arc melted" and "powder samples were ground from the as-cast
   ↪ ingots".
6  In the experimental details, it says the alloys were "arc melted" and that they
   ↪ confirmed a single "bcc structure". And there's a specific lattice constant
   ↪ for TiVNbTa: 3.2206 (9) Å.
```

7 Now, into the "Results and discussion." TiVNbTa is being discussed a lot, and the  
 ↳ lattice constant is repeated, so that is another confirmation of its bcc  
 ↳ structure. TiVNbMoTa is also mentioned. I see comparisons between the two,  
 ↳ which provides a lattice constant for TiVNbMoTa. Other alloys identified are  
 ↳ "TiVNbZr", "TiVNbMo" (this needs careful attention, as it may or may not be  
 ↳ the same as TiVNbMoTa. For now, I'm assuming it's a separate 4-element  
 ↳ alloy), and more mentions of NiCoFeCr and NiCoFeCrPd (as comparisons). The  
 ↳ general condition given is the same for TiVNbTa, TiVNbMoTa, TiVNbZr, and  
 ↳ TiVNbMo: Arc melted from the mixture. "Powder samples were ground from the  
 ↳ as-cast ingots". I will use the "as-cast" condition, as that is the intrinsic  
 ↳ state of the alloy that the properties are associated with.

8 **\*\*Final Data Points and JSON Output\*\***

9 I've carefully examined all the pertinent text, ensuring I understand the  
 ↳ preparation methods, the alloy's conditions for property measurements, and  
 ↳ the meaning of each parameter. After all that analysis, I'm ready to craft  
 ↳ the JSON objects, and I've decided to exclude MoNbTaW from the list of  
 ↳ *\*primary alloys analyzed in this paper\**.

10 Here's my final list:

11 **\*\*1. TiVNbTa\*\***

```
12 ```json
13 {
14     "name": "TiVNbTa",
15     "nominal_composition": "Ti1.0V1.0Nb1.0Ta1.0",
16     "measured_composition": "Not found",
17     "lattice_constant": "3.221 |\\AA{}|",
18     "phases": "bcc solid-solution structure",
19     "alloy_condition": "As-Cast",
20     "doi": "10.1016/j.jallcom.2020.155970"
21 }
22 ```
```

```

23  **2. TiVNbMoTa**
24  ```json
25  {
26    "name": "TiVNbMoTa",
27    "nominal_composition": "Ti1.0V1.0Nb1.0Mo1.0Ta1.0",
28    "measured_composition": "Not found",
29    "lattice_constant": "3.197 |\\AA{ }|",
30    "phases": "bcc solid-solution structure",
31    "alloy_condition": "As-Cast",
32    "doi": "10.1016/j.jallcom.2020.155970"
33  }
34  ```
35  **3. NiCoFeCrMn**
36  ```json
37  {
38    "name": "NiCoFeCrMn",
39    "

```

---

**Figure S11:** The extended reasoning history from Gemini 2.5 Flash with dynamic thinking budget for the Zhang et al. [9] publication showing its internal reasoning process before generating the final extraction output..

## S6. EXTENDED REASONING USING CLAUDE 4.5 SONNET MODEL

```
1  Let me carefully read through the PDF to extract information about all
   ↪  high-entropy alloys discussed in the results section.
2  From the Results and Discussion section, I can identify the following alloys:
3  1. **TiVNbTa** - mentioned in Fig. 1a and b, neutron diffraction profiles
4     - Lattice constant at room temperature: 3.2206 (9) Å
5     - Average volume: 16.70 (2) Å3/atom
6     - Structure: bcc
7     - Nominal composition: Ti1.0V1.0Nb1.0Ta1.0
8  2. **TiVNbMoTa** - mentioned alongside TiVNbTa
9     - Structure: bcc
10    - Nominal composition: Ti1.0V1.0Nb1.0Mo1.0Ta1.0
11  3. **NiCoFeCrMn** - mentioned as a comparison fcc alloy
12    - Debye-Waller factor at room temperature: 0.40 Å3
13    - Structure: fcc
14    - Nominal composition: Ni1.0Co1.0Fe1.0Cr1.0Mn1.0
15  4. **TiVNbZr** - mentioned in the text
16    - Structure: bcc
17    - Nominal composition: Ti1.0V1.0Nb1.0Zr1.0
18  5. **TiVNbMo** - mentioned in the text
19    - Structure: bcc
20    - Nominal composition: Ti1.0V1.0Nb1.0Mo1.0
21  All alloys appear to be from arc-melted/as-cast condition based on the
   ↪  experimental details.
22  DOI: 10.1016/j.jallcom.2020.155970
23  Let me extract specific information for each alloy from the results section.
```

---

**Figure S12:** The extended reasoning history from Claude 4.5 Sonnet with 1024 thinking budget for the Zhang et al. [9] publication showing its internal reasoning process before generating the final extraction output.

## S7. POTENTIAL IMPROVEMENTS

We identify four potential strategies for improving data extraction reliability.

Strategy 1: Expand Training Set Diversity. The optimization process would benefit from expert-labeled papers representing greater diversity in: (i) authorship, (ii) target applications and material systems, (iii) journal formatting conventions, and (iv) data presentation styles (text vs. tables vs. figures). Increased diversity would provide the prompt optimization algorithm with broader exposure to edge cases, ambiguous phrasings, and varied reporting conventions, improving generalization to the full literature collection. Zheng et al. [10] made a similar recommendation in their study.

Strategy 2: Implement Output-Level “Gradient” Optimization. We can extend the TEXTGRAD optimization framework to include a Module 4 that uses output-level “gradients” in addition to prompt-level optimization. As demonstrated in Section 4, the EvaluatePdfOutputLoss function successfully identifies many extraction errors in generated outputs. Implementing an additional optimization loop that iteratively refines outputs based on these loss signals could enable automatic error correction. However, this approach has two limitations: (i) when the LLM rationalizes its errors (where the model asserted that 0.319 Å was correct), the loss function fails to generate corrective “textual gradients”, maintaining the error, and (ii) additional optimization is costly as each refinement requires multiple API calls to commercial LLM services.

Strategy 3: Prioritize Original Publisher PDFs Over XML Reconstructions. We identify that there is value in using publisher-provided PDFs rather than PDFs reconstructed from XML sources. While XML-to-PDF reconstruction successfully preserved text and tabular data for most papers, formatting fidelity was inconsistent. This was especially true for publications with equations, special symbols, and complex multi-column tables. These formatting artifacts can potentially impair LLM extraction performance. A representative example from Cui et al. [8] illustrates this impact. Extraction from the XML-reconstructed PDF identified only three of six HEA compositions (recall = 0.50), with the loss function (Figure S10 in SI) confirming the missed entries. In contrast, the same extraction pipeline applied to the publisher’s original PDF correctly identified all six compositions in a single pass, indicating that formatting quality directly affects extraction reliability. The exact mechanism that

contributes to this improvement needs further investigation.

Strategy 4: Leverage Advances in LLM Model Capabilities. LLM models continue to improve rapidly, with each generation showing enhanced reasoning, improved adherence to prompt specifications, and multimodal understanding [11, 12]. Future LLM models may substantially improve extraction performance through better contextual understanding, reduced hallucination rates, and improved handling of complex scientific content. Our cross-model evaluation (discussed in Testing Prompt Transferability subsection in the main manuscript) demonstrates this trend, with newer models achieving superior performance even with unoptimized prompts. In addition, retrieval-augmented generation (RAG) offers another promising approach to reduce semantic hallucination by ensuring LLM outputs are based on actual document content rather than model memory [13]. Nonetheless, the high cost of commercial LLM APIs could restrict their broad use for large-scale data extraction in resource-constrained research environments. Fine-tuning open-source LLMs presents a promising and cost-effective alternative that deserves further exploration.

## S8. PERFORMANCE OF THE TRAINED ML MODELS IN PREDICTING LATTICE CONSTANTS

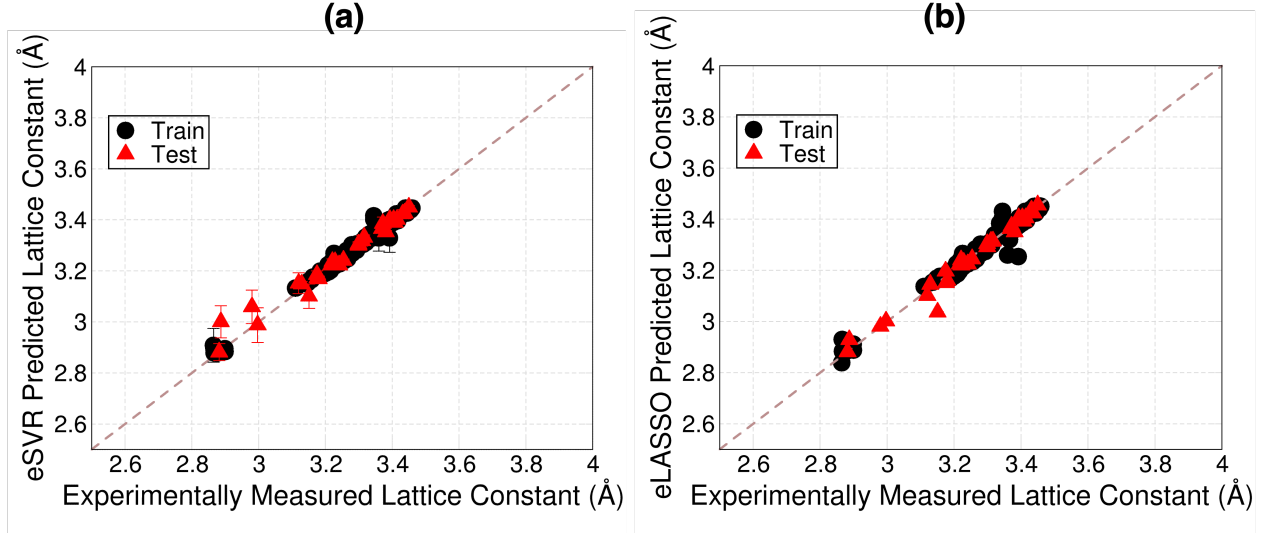

**Figure S13:** Parity plot comparing (a) eSVR-predicted (y-axis) and (b) eLASSO-predicted lattice constants (y-axis) against experimental lattice constants (x-axis) for LLM-extracted as-cast single-phase BCC HEAs. Data points falling on the diagonal dashed line ( $y = x$ ) represents perfect prediction. Filled black circles denote training set data (127 data points), and filled red triangles indicate test set data (32 data points). Error bars represent prediction uncertainty quantified as the standard deviation across the 100 ensemble SVR models in (a), and 1000 ensemble LASSO models in (b). Strong clustering along the diagonal for both training and test sets demonstrates good model generalization (test  $R^2 = 0.969$  and  $0.974$  for eSVR and eLASSO, respectively).

## S9. SUGGESTED STEPS PRIOR TO PERFORMING DOWNSTREAM TASKS

Based on the lessons learned from our detailed analysis of the as-cast single-phase BCC HEAs, we recommend the following steps prior to performing any downstream tasks with the extracted lattice constants.

- Randomly select  $n$  publications (where the exact value of  $n$  depends on the budget) and verify that the LLM has accurately extracted the lattice constants from those publications. For convenience, the DOI is provided in the same row as the corresponding lattice constant data. Ideally, both precision and recall should be close to 1.
- If the budget allows, conduct the `ExtractPDFOutputLoss` analysis for those  $n$  publications to evaluate the accuracy of the extracted outputs.
- Use the `Check_Composition_Consistency.py` provided with the source code to verify compositional information (the GitHub link is given in the Code Availability section in the main manuscript). Manually check if the L1 distance ( $D_{L1}$  in Equation 4 in the main manuscript) or cosine similarity (CosSim in Equation 5 in the main manuscript) are unusual. This utility python script has provided useful parsing strategies that normalizes composition and will flag rows with inconsistent compositions.

## S10. PSEUDOCODE FOR THE ITERATIVE PROMPT OPTIMIZATION

The pseudocode is shown in Figure S14.

### Iterative Prompt Optimization

```
Inputs: train_loader
          prompt  $\leftarrow$  initial_prompt
          model  $\leftarrow$  LLM(prompt)
          optimizer  $\leftarrow$  TEXTUALGRADIENTDESCENT({prompt})
          loss_fn  $\leftarrow$  EVALUATEPDFEXTRACATIONLOSS()
1: for epoch  $\leftarrow$  1 to  $E$  do
2:   for each (batch $x$ , batch $y$ ) in train_loader do
3:      $\mathcal{L} \leftarrow []$ 
4:     for each ( $x, y$ ) in (batch $x$ , batch $y$ ) do
5:        $\hat{y} \leftarrow$  model( $x$ )
6:        $\ell \leftarrow$  loss_fn(prompt,  $x, \hat{y}, y$ )
7:       append( $\mathcal{L}, \ell$ )
8:     end for
9:      $L \leftarrow \sum_{\ell \in \mathcal{L}} \ell$ 
10:    BACKPROPAGATE( $L$ )
11:    UPDATEPARAMETERS(optimizer)
12:  end for
13: end for
```

**Figure S14:** Pseudocode for iterative prompt optimization (Module 2) based on the TEXTGRAD framework [14]. The inputs are:  $x$  (original PDF),  $y$  (expert-labeled ground truth data), and  $\hat{y}$  (LLM-generated output). The training data are loaded in batches via `train_loader`, which provides batches of PDFs (batch <sub>$x$</sub> ) and corresponding expert labels batch <sub>$y$</sub> . For each ( $x, y$ ) pair in a batch, the PDF  $x$  is processed by the LLM using the current prompt to generate  $\hat{y}$ , and the `EvaluatePdfExtractionLoss` function computes the loss  $\ell$  by comparing  $\hat{y}$  to the expert label  $y$ . Individual losses within the batch are accumulated in list  $\mathcal{L}$  and summed to produce batch loss  $L$  (line 9). The loss is then backpropagated through the prompt using textual gradient descent, and the prompt parameters are updated by the optimizer. This process repeats for  $E$  epochs across all training batches. For implementation details, see Yuksekogonul et al. [14].

## S11. PROMPTS USED FOR THE LOSS FUNCTION DURING PROMPT OPTIMIZATION

```
1 Below is the output from a data extraction task for a given PDF file, the PDF
   ↪ data, and the result from human of this task.
2         You need to evaluate the output and the result from human.
3         ONLY compare presented entries, do not perform task yourself.
4 Is the output matches with human results? i.e., Does the reported parameter match
   ↪ with the PDF data and the human?
5 i.e., does the number of material matches with PDF and human annotation? Does the
   ↪ lattice constant matches with the PDF and human annotation?
6         Say match if it does, otherwise say it doesn't match.
7         Be super consice.
```

---

**Figure S15:** Prompts for the loss function during prompt optimization (Module 2).

1 Below is the output from a data extraction task for a given PDF file, and the PDF  
↳ itself.

2 You need to evaluate the output according to the provided PDF for each extracted  
↳ material, be super concise:

3 Does the output matches the format provided in the question? Answer yes or no.

4 Are the extract material high-entropy alloys? Answer yes or no.

5 Are the alloy composition in the output correct and reflect the material? Answer  
↳ yes or no.

6 Are the lattice constants value in the output formatted in angstrom? Answer yes  
↳ or no.

7 Are the lattice constants in the output truly the lattice constant of the  
↳ material not others? Answer yes or no.

8 Are the phase information in the output correct and reflect the material? Answer  
↳ yes or no.

9 Are the alloy condition in the output correct and reflect the material? Answer  
↳ yes or no.

10 Is the DOI in the output matches with the original paper? Answer yes or no.

11 Is there any HEA high-entropy alloys missed in the provided ouput? yes or no.

---

**Figure S16:** Prompts for the loss function for output evaluation.

## S12. DEFINITION OF CONFUSION MATRIX FOR RETRIEVAL EVALUATION

The confusion matrix, which defines true positives (TP), true negatives (TN), false positives (FP), and false negatives (FN), is presented in Table S3 below [15, 16].

**TABLE S3:** Definition of various terms in the confusion matrix for information retrieval evaluation.

|                      | <b>Relevant</b>      | <b>Non-relevant</b>  |
|----------------------|----------------------|----------------------|
| <b>Retrieved</b>     | True Positives (TP)  | False Positives (FP) |
| <b>Not Retrieved</b> | False Negatives (FN) | True Negatives (TN)  |

### **S13. DESCRIPTOR SELECTION FOR THE DOWNSTREAM MACHINE LEARNING TASK**

The descriptor selection pipeline employs Recursive Feature Elimination with Cross-Validation (REFCV), as implemented in `scikit-learn`[17]. This module selects descriptors by iteratively removing the least important ones through a recursive process. This method is commonly applied in various machine learning tasks in the literature [18–20]. In our study, we utilize REFCV in conjunction with `RandomForestRegression` [21], employing a three-fold cross-validation strategy (CV=3). We started with 36 descriptors and the REFCV approach downselected six descriptors for training the ML models.

## REFERENCES

- [1] Allen Institute for AI. Asta: Agentic AI research assistant. <https://asta.allen.ai>, 2025. Accessed 4 October 2025.
- [2] Mujin Yang, Chao Huang, Jiajia Han, Haichen Wu, Yilu Zhao, Tao Yang, Shenbao Jin, Chenglei Wang, Zhou Li, Ruiying Shu, Cuiping Wang, Huanming Lu, Gang Sha, and Xingjun Liu. Development of the high-strength ductile ferritic alloys via regulating the intragranular and grain boundary precipitation of G-phase. *Journal of Materials Science & Technology*, 136:180–199, 2023.
- [3] S. Pan, J.Q. Zhang, B.B. He, and M.X. Huang. High strain gradient induced nanograin in a coCrNiV medium entropy alloy with lamellar carbide. *Materials Science and Engineering: A*, 852:143692, 2022.
- [4] C.L. Wu, S. Zhang, C.H. Zhang, H. Zhang, and S.Y. Dong. Phase evolution and cavitation erosion-corrosion behavior of FeCoCrAlNiTi<sub>0.5</sub> high entropy alloy coatings on 304 stainless steel by laser surface alloying. *Journal of Alloys and Compounds*, 698:761–770, 2017.
- [5] Jongun Moon, Elena Tabachnikova, Sergii Shumilin, Tetiana Hryhorova, Yuri Estrin, Jamieson Brechtel, Peter K. Liaw, Wenqing Wang, Karin A. Dahmen, Alireza Zargaran, Jae Wung Bae, Hyeon-Seok Do, Byeong-Joo Lee, and Hyoung Seop Kim. Deformation behavior of a co-Cr-Fe-Ni-Mo medium-entropy alloy at extremely low temperatures. *Materials Today*, 50:55–68, 2021.
- [6] David Piorunek, Jan Frenzel, Niels Jöns, Christoph Somsen, and Gunther Eggeler. Chemical complexity, microstructure and martensitic transformation in high entropy shape memory alloys. *Intermetallics*, 122:106792, 2020.
- [7] Yiling Jiang, Haibo Tang, Zhuo Li, Dongdong Zheng, and Yuxuan Tu. Additive manufactured Mg-Gd-Y-Zr alloys: Effects of Gd content on microstructure evolution and mechanical properties. *Additive Manufacturing*, 59:103136, 2022.
- [8] Peng Cui, Yimo Ma, Lijun Zhang, Mengdi Zhang, Jiantao Fan, Wanqing Dong, Pengfei Yu, and Gong Li. Microstructure and mechanical behaviors of CoFeNiMnTi<sub>x</sub>Al<sub>1-x</sub> high entropy alloys. *Materials Science and Engineering: A*, 731:124–130, 2018.

- [9] F.X. Zhang, Y. Tong, M. Kirkham, A. Huq, H. Bei, W.J. Weber, and Y. Zhang. Structural disorder, phase stability and compressibility of refractory body-centered cubic solid-solution alloys. *Journal of Alloys and Compounds*, 847:155970, 2020.
- [10] Zhiling Zheng, Oufan Zhang, Christian Borgs, Jennifer T Chayes, and Omar M Yaghi. Chat-GPT chemistry assistant for text mining and the prediction of MOF synthesis. *Journal of the American Chemical Society*, 145(32):18048–18062, 2023.
- [11] Long Ouyang, Jeffrey Wu, Xu Jiang, Diogo Almeida, Carroll Wainwright, Pamela Mishkin, Chong Zhang, Sandhini Agarwal, Katarina Slama, Alex Ray, et al. Training language models to follow instructions with human feedback. *Advances in neural information processing systems*, 35:27730–27744, 2022.
- [12] Mian Zhang, Shujian Liu, Sixun Dong, Ming Yin, Yebowen Hu, Xun Wang, Steven Ma, Song Wang, Sathish Reddy Indurthi, Haoyun Deng, et al. Complex logical instruction generation. *arXiv preprint arXiv:2508.09125*, 2025.
- [13] Patrick Lewis, Ethan Perez, Aleksandra Piktus, Fabio Petroni, Vladimir Karpukhin, Naman Goyal, Heinrich Küttler, Mike Lewis, Wen-tau Yih, Tim Rocktäschel, et al. Retrieval-augmented generation for knowledge-intensive nlp tasks. *Advances in neural information processing systems*, 33:9459–9474, 2020.
- [14] Mert Yuksekgonul, Federico Bianchi, Joseph Boen, Sheng Liu, Pan Lu, Zhi Huang, Carlos Guestrin, and James Zou. Optimizing generative AI by backpropagating language model feedback. *Nature*, 639(8055):609–616, 2025.
- [15] Xin Wang, Anshu Raj, Matthew Luebke, Haiming Wen, Shuozhi Xu, and Kun Lu. Reliable End-to-End Material Information Extraction from the Literature with Source-Tracked Multi-Stage Large Language Models, 2025.
- [16] Christopher D. Manning, Prabhakar Raghavan, and Hinrich Schütze. *Introduction to Information Retrieval*. Cambridge University Press, 2008.
- [17] F. Pedregosa, G. Varoquaux, A. Gramfort, V. Michel, B. Thirion, O. Grisel, M. Blondel, P. Prettenhofer, R. Weiss, V. Dubourg, J. Vanderplas, A. Passos, D. Cournapeau, M. Brucher, M. Perrot, and E. Duchesnay. Scikit-learn: Machine Learning in Python. *Journal of Machine Learning Research*, 12:2825–2830, 2011.

- [18] Junya Wang, Pengcheng Xu, Xiaobo Ji, Minjie Li, and Wencong Lu. Feature Selection in Machine Learning for Perovskite Materials Design and Discovery. *Materials*, 16, 2023.
- [19] Sofia Sheikh, Brent Vela, Vahid Attari, Xueqin Huang, P. Morcos, James Hanagan, Cafer Acemi, Ibrahim Karaman, A. Elwany, and Raymundo Arroyave´. Exploring chemistry and additive manufacturing design spaces: a perspective on computationally-guided design of printable alloys. *Materials Research Letters*, 12:235 – 263, 2024.
- [20] Elliot H. E. Farrar and Matthew N. Grayson. Machine learning and semi-empirical calculations: a synergistic approach to rapid, accurate, and mechanism-based reaction barrier prediction. *Chemical Science*, 13:7594 – 7603, 2022.
- [21] Kevin Maik Jablonka, Daniele Ongari, Seyed Mohamad Moosavi, and Berend Smit. Big-Data Science in Porous Materials: Materials Genomics and Machine Learning. *Chemical Reviews*, 120:8066 – 8129, 2020.
